# Supplementary material for: TimeMixer++: A General Time Series Pattern Machine for Universal Predictive Analysis
Source: arXiv:2410.16032 source file (2025-05-19)
Supplement: Supplementary file 1 [file additional_results.tex]

% \section{Additional Experiments}
% \label{sec:more_experiments}


% \vspace{-1mm}
% \begin{table}[H]
% \renewcommand\arraystretch{1.2}
% \begin{center}
% \caption{Cross-domain Zero-shot learning results. We follow the same protocol as \citep{zhou2023one} and report results from \citep{liu2024autotimes}. $M4\rightarrow M3$ means training the model on the datasets of M4 and then evaluating
% on M3, and vice versa.}
% \label{tab:zero-shot-cross}
% \vspace{-3mm}
% \resizebox{\columnwidth}{!}{
%   \begin{threeparttable}
%   \begin{small}
% \setlength\tabcolsep{4pt}
% \begin{tabular}{c|cccccccccc}
% \toprule
% \multirow{2}{*}{\textbf{Methods}} & \textbf{TimeMixer++} & \textbf{FPT} & \textbf{DLinear} & \textbf{PatchTST} & \textbf{AutoTimes} & \textbf{TimesNet} & \textbf{Nsformer} & \textbf{FEDformer} & \textbf{Informer} & \textbf{Reformer} \\
% % \midrule
%  & \citeyearpar{zhou2023one} & \citeyearpar{zhou2023one} & \citeyearpar{dlinear} & \citeyearpar{patchtst} & \citeyearpar{liu2024autotimes} & \citeyearpar{wu2022timesnet} & \citeyearpar{Liu2022NonstationaryTR} & \citeyearpar{zhou2022fedformer} & \citeyearpar{zhou2021informer} & \citeyearpar{kitaev2020reformer} \\
% \midrule
% $M4 \rightarrow M3$ & \textbf{12.49} & 13.06 & 14.03 & 13.06 & 12.75 & 14.17 & 15.29 & 13.53 & 15.82 & 13.37 \\
% $M3 \rightarrow M4$ & \textbf{12.756} & 13.125 & 15.337 & 13.228 & 13.036 & 14.553 & 14.327 & 15.047 & 19.047 & 14.092 \\
% \bottomrule
% \end{tabular}
% \end{small}
% \end{threeparttable}
% }
% \end{center}
% \end{table}
% \vskip -0.1in

% \red{As shown in Table.~\ref{tab:zero-shot-cross}, \method demonstrates the best performance across both tasks, outperforming other methods and showcasing its superior ability to generalize temporal patterns without task-specific training. \method consistently delivers the lowest errors, with improvements ranging from 2\% to 33\% compared to competing methods. }

% \vspace{-2mm}
% \begin{table}[H]
% \renewcommand\arraystretch{1.2}
% \begin{center}
% \caption{Inference time comparison across models on long-term forecasting using ETTm1. The results are reported in milliseconds per iteration (ms/iter). Additional efficiency estimations are provided in Section~\ref{sec:efficiency}.}
% \label{tab:inference-time}
% % \vspace{-3mm}
% \resizebox{\columnwidth}{!}{
%   \begin{threeparttable}
%   \begin{small}
% \setlength\tabcolsep{4pt}
% \begin{tabular}{c|cccccccc}
% \toprule
% \textbf{Methods} & \textbf{TimeMixer++} & \textbf{iTransformer} & \textbf{PatchTST} & \textbf{FEDformer} & \textbf{TimeMixer} & \textbf{TIDE} & \textbf{TimesNet} & \textbf{SCINet} \\
% \midrule
% \textbf{Inference Time} & 90 & 130 & 105 & 240 & 90 & \textbf{85} & 160 & 150 \\
% \bottomrule
% \end{tabular}
% \end{small}
% \end{threeparttable}
% }
% \end{center}
% \end{table}
% \vskip -0.1in

% \red{As shown in Table.~\ref{tab:inference-time}, \method demonstrates exceptional inference efficiency compared to baseline models. With an inference speed of 90 ms/iter, \method matches the performance of TiDE and outperforms other models, such as TimesNet (160 ms/iter) and SCINet (150 ms/iter), achieving a speedup of 43.75\% and 40\%, respectively.
% }




% \vspace{-1mm}
% \begin{table}[H]
% \renewcommand\arraystretch{1.2}
% \begin{center}
% \caption{Comparison of MLP-mixing and Attention-mixing on forecasting tasks. Results are reported for Mean Squared Error (MSE) and Mean Absolute Error (MAE).}
% \label{tab:mlp-vs-attention}
% \vspace{2mm}
% \begin{threeparttable}
% \begin{small}
% \setlength\tabcolsep{10pt} % Adjust column spacing
% \begin{tabular}{c|cc|cc}
% \toprule
% \textbf{Method} & \multicolumn{2}{c|}{\textbf{MLP-mixing}} & \multicolumn{2}{c}{\textbf{Attention-mixing}} \\
% Horizon & MSE & MAE & MSE & MAE\\
% \midrule
% 96  & 0.587 & 0.271 & 0.412 & 0.297 \\
% 192 & 0.599 & 0.292 & 0.434 & 0.289 \\
% 336 & 0.627 & 0.346 & 0.452 & 0.297 \\
% 720 & 0.641 & 0.377 & 0.483 & 0.311 \\
% \bottomrule
% \end{tabular}
% \end{small}
% \end{threeparttable}
% \end{center}
% \end{table}
% \vskip -0.1in


% \red{We evaluated two channel mixing strategies, MLP-mixing and attention-mixing, on the Traffic dataset, which comprises 862 channels. The input context length is fixed at 96, and the prediction horizons are set to \{96, 192, 336, 720\}. From the table, we observe that attention-mixing consistently outperforms MLP-mixing in terms of MSE for all prediction horizons. For example, at the 96-step prediction horizon, attention-mixing achieves an MSE of 0.412, which is a 29.8\% improvement over MLP-mixing. Similarly, at the 720-step horizon, the MSE reduction with attention-mixing is 24.6\%.
% }
